# Supplementary material for: Argus: From Rasterized-Camera Self-Play to Real-Camera Driving
Source: arXiv:2611.37876 source file (2026-11-27)
Supplement: Supplementary file 1 [file X_appendix.tex]

\clearpage
\twocolumn[\centering\Large\textbf{\thetitle}\\\vspace{0.5em}Appendix\\\vspace{1.0em}]
\appendix

\addtocontents{toc}{\protect\setcounter{tocdepth}{2}}
{\makeatletter
\def\tocskipdot\hskip -1em.#1{\ifx#1\nobreakspace\expandafter\@gobble\fi}%
\def\numberline#1{\hb@xt@\@tempdima{#1.\hfil}\@ifnextchar\hskip\tocskipdot{}}%
\tableofcontents}

\input{sec/A_implementation}
\input{sec/B_protocol}
\input{sec/C_results}

\clearpage
